# Supplementary material for: Single acquisition reconstruction of nonlinear susceptibility and Raman tensors at the diffraction limit
Source: arXiv:2602.03196 ancillary file (2026-04-29)
Supplement: Supplementary file 1 [file Supplementary.pdf]

# Supporting Information:

## Simultaneous measurement of Raman and nonlinear optical tensors

Volodymyr Multian,<sup>†,‡,¶</sup> Luigi Bonacina,<sup>‡</sup> and Jérémie Teyssier<sup>\*,†</sup>

<sup>†</sup>*Department of Quantum Matter Physics, University of Geneva, 24 Quai Ernest Ansermet, Geneva CH-1211, Switzerland*

<sup>‡</sup>*Nonlinear BioImaging Lab, Department of Applied Physics, University of Geneva 24 Quai Ernest Ansermet, Geneva CH-1211, Switzerland*

<sup>¶</sup>*Photon Processes Department, Institute of Physics of NAS of Ukraine. Prospect Nauky, 46, Kyiv-03028, Ukraine.*

E-mail: jeremie.teyssier@unige.ch

## 1 Detailed scheme of the experimental setup

Scheme of Raman/SHG microscope with 3D rendering of the setup presented in figure S1.

## 2 Polarization resolved ray tracing

Reconstructing images captured by the CCD in the Fourier plane involves analyzing the propagation of the polarized pump beam from the source, through the objective to the sample, as well as the backward propagation of the emitted SHG signal to the CCD. Although this task can be solved precisely with complex finite element approaches or algorithms for

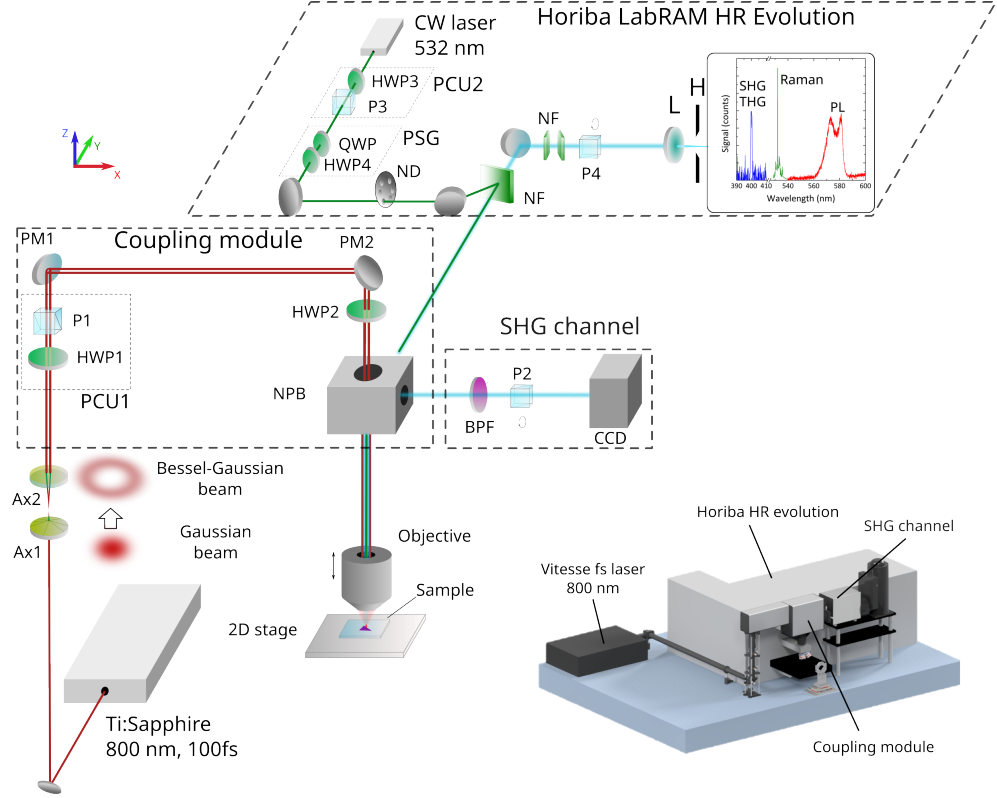

Figure S1: Schematic representation of Raman/SHG microscope. Ax1,2 - axicons, HWP1-4 - half-wave plates, QWP - quarter-wave plate, P1-4 - polarizers, PM1,2 - mirrors with piezo actuators, ND - neutral density filters, PCU1,2 - power control unit, PSG - polarization state generator, NF - notch filter, BPF - band pass filter, NPB - non polarizing beam splitter/multiplexer module, CCD - LN cooled 2D charged coupled device, L - focusing lens, H - motorized hole

the simulation of vector beams propagation<sup>S1-S4</sup> with a defined set of initial parameters and optical geometry, it would require excessive computational resources to fit the experimental data. For this reason, we opted for ray tracing, which is sufficiently accurate to model the intensity distribution at the Fourier plane while being less resource-demanding.

In our analysis, we set-up a ray tracing for a grid of  $N$  beamlets characterized by complex beam parameter  $q$  that start at point  $\vec{r}$  ( $N \times 3$ ) and propagate in the direction of wave vector  $\vec{k}$  defined by the unit vector  $\hat{k}$  ( $N \times 3$ ) in laboratory basis. Each of the  $N$  beamlet will contain information about the  $K$  polarization states expressed by the 3D Jones vectors  $\vec{E}$  ( $K \times N \times 3$ ). Set  $(\vec{r}, q, \hat{k}, \vec{E})$  together with total optical path  $OPL$ , we will call "polarized beamlet"

that contains full information about the polarized light in 3D space. Each parameter in the practical realization of the model will be represented in tensor form to vectorize the calculations, while the mathematical description will be shown below for a single beamlet.

## General concepts

### P matrix

Propagation of polarized ray at  $m$ -th step of ray tracing with wave vector  $\hat{k}^m$  and field  $\vec{E}^m$  through a polarizing optical element can be calculated with the use of P-matrix approach:<sup>S5</sup>

$$\vec{E}^{m+1} = P^m \vec{E}^m. \quad (1)$$

25

If the optical element does not refract the ray and is aligned along  $\hat{k}$ , it can be described by  $P$  matrix in the form of a 2D Jones matrix  $J$ :

$$P = \begin{pmatrix} J & 0 \\ 0^T & 1 \end{pmatrix} \quad (2)$$

In this way, we can represent in 3D space polarizing optical elements like a linear diattenuator  $J^D$ , linear retarder  $J^R$ , or general polarizing optical elements  $J^G$ :

$$J^D = \begin{pmatrix} a & 0 \\ 0 & b \end{pmatrix}, \quad (3)$$

$$J^R = \begin{pmatrix} e^{-i\phi_x} & 0 \\ 0 & e^{-i\phi_y} \end{pmatrix}, \quad (4)$$

$$J^G = \begin{pmatrix} j_{00} & j_{01} \\ j_{10} & j_{11} \end{pmatrix}, \quad (5)$$

where  $a, b$  - diattenuation coefficients,  $\phi_{x,y}$  - phases for fast and slow axes,  $j_{ij}$  - Jones matrix elements defined by properties of the optical element.

### Transformation of **P** matrix

To propagate the electrical field  $\vec{E}$  through the optical system, we need to calculate  $P$  matrices for each element, taking into account its orientation in 3D space and the orientation of the wave vector  $\hat{k}$  at each interface.

The transformation of the tensor  $\mathcal{M}$  of rank  $V$  by an arbitrary transformation matrix  $\mathcal{T}$  can be performed according to the general transformation approach:

$$\mathcal{M}_{a\dots x}^{m+1} = \prod_2^V \mathcal{T}_{a\alpha} \mathcal{T}_{b\beta} \dots \mathcal{T}_{x\omega} \mathcal{M}_{\alpha\dots\omega}^m. \quad (6)$$

This approach can be used for rotation of  $P$  in 3D space by rotation matrix  $R$ :

$$P_{ij}^{m+1} = R_{i\alpha} R_{j\beta} P_{\alpha\beta}^m. \quad (7)$$

The propagation of the ray through the interface characterized by normal  $\hat{N}$  and matrix

40  $P_m$  that change the wave vector from  $\hat{k}^m$  to  $\hat{k}^{m+1}$  can be described as:

$$P^{m+1} = O^{m+1} P^m (O^m)^{-1}, \quad (8)$$

41 where basis transformation matrices  $O^m$  and  $O^{m+1}$  are constructed from unit vectors  $\hat{s}$ ,  $\hat{p}$  and  
42  $\hat{k}$ :

$$O^m = \left( \hat{s}^m, \hat{p}^m, \hat{k}^m \right), \quad (9)$$

$$O^{m+1} = \left( \hat{s}^{m+1}, \hat{p}^{m+1}, \hat{k}^{m+1} \right). \quad (10)$$

43 Unit vectors  $\hat{s}$  and  $\hat{p}$  can be determined from wave vectors and normal  $\hat{N}$  as follows:

$$\hat{s} = \frac{\hat{k} \times \hat{N}}{|\hat{k} \times \hat{N}|}, \hat{p} = \frac{\hat{k} \times \hat{s}}{|\hat{k} \times \hat{s}|}. \quad (11)$$

44 For the propagation of the wave with field  $\vec{E}$  and wave vector  $\hat{k}$  through such an interface,  
45 the optical path length OPL has to be calculated:

$$OPL = nl\hat{k} \cdot \hat{S}, \quad (12)$$

46 where  $n$  is a refractive index,  $l$  distance propagated inside the interface,  $\hat{S}$  the Pointing unit  
47 vector, which in the case of isotropic media is equal to the  $\hat{k}$  inside the interface. This allows  
48 us to write the resulting  $\tilde{P}$  matrix for the interface in the following expression:

$$\tilde{P} = (P - S_D) e^{ikOPL} + S_D, \quad (13)$$

49 where  $S_D = \hat{S}_{out} \hat{S}_{in}^T$  is  $S$  dyad matrix. In this way we can write the  $P$  matrix for refrac-  
50 tion/reflection at the interface based on Jones matrix for a diattenuator Eq. 3. Diattenuation  
51 coefficients  $a$ ,  $b$  in this case will correspond to the Fresnel reflection ( $r^s, r^p$ ) and transmission  
52 ( $t^s, t^p$ ) coefficients<sup>S6</sup> :

$$r^p = \frac{\tan(\theta^m - \tilde{\theta}^{m+1})}{\tan(\theta^m + \tilde{\theta}^{m+1})}, \quad r^s = -\frac{\sin(\theta^m - \tilde{\theta}^m)}{\sin(\theta^m + \tilde{\theta}^{m+1})} \quad (14)$$

$$t^p = \frac{n^m}{n^{m+1}}(r^p + 1), \quad t^s = r^s + 1, \quad (15)$$

where  $n^{m-1,m}$  – refractive indexes of input/output media,  $r^{s,p}$  - reflection coefficients for  $s$  and  $p$  polarization. The incidence and refraction angles  $\theta$  and  $\tilde{\theta}$  can be calculated from Snell's law:

$$\theta^m = \cos^{-1}(\hat{k}^m \cdot \hat{N}^m) \quad (16)$$

$$\tilde{\theta}^{m+1} = \sqrt{1 - \left(\frac{n^m}{n^{m+1}}\right)^2 (1 - \cos^2 \theta^m)}. \quad (17)$$

$P^{ref}$  matrix can be constructed from  $J^D$  according to Eq.2. Refracted and transmitted wave vectors can be obtained from the initial  $\hat{k}$ :

$$\hat{k}^{r,m+1} = \hat{k}^m - 2(\hat{k}^m \cdot \hat{N}^m)\hat{N}^m \quad (18)$$

$$\hat{k}^{t,m+1} = \frac{n^m}{n^{m+1}}\hat{k}^m - \left(\frac{n^m}{n^{m+1}}\cos\theta^{m+1} - \cos\tilde{\theta}^{m+1}\right)\hat{N}^m, \quad (19)$$

Calculated reflected and transmitted  $\hat{k}^r$  and  $\hat{k}^t$  now can be used to transform the  $P$  matrix of the interface according to Eq.7. Finally propagation of the wave after the interface can be performed with Eq.13 and Eq.2.

## Propagation through ABCD system

According to the ray transfer matrix approach, the propagation of the beamlet characterized by position  $\vec{r}$ , chief ray  $\hat{k}$  and complex parameter  $q$  can be calculated with ABCD matrices.<sup>S7</sup> The algorithm of calculation consists of the following steps:

- propagation of the beamlet to the entrance pupil of the optical system;
- calculation of real ray  $[\check{r}, \tan \check{\theta}]$  from 3D coordinates of vector  $\vec{r}$  and  $\hat{k}$ , where  $\check{r}$  is  $\vec{r}$  projected on the plane of the optical element, and  $\check{\theta}$  - angle between the axis of optical element and  $\hat{k}$ ;
- calculation of complex ray  $[q, 1]$ ;
- propagation through ABCD system by multiplication of input rays by corresponding ABCD matrix;
- extraction of 3D coordinate of the beamlet, wave vector and complex beam parameter;
- propagation of the field  $\vec{E}$  by calculation of  $P$  matrices for each interface from  $\hat{k}$  vectors and optical path lengths.

## Delivering polarized light from the source to the sample

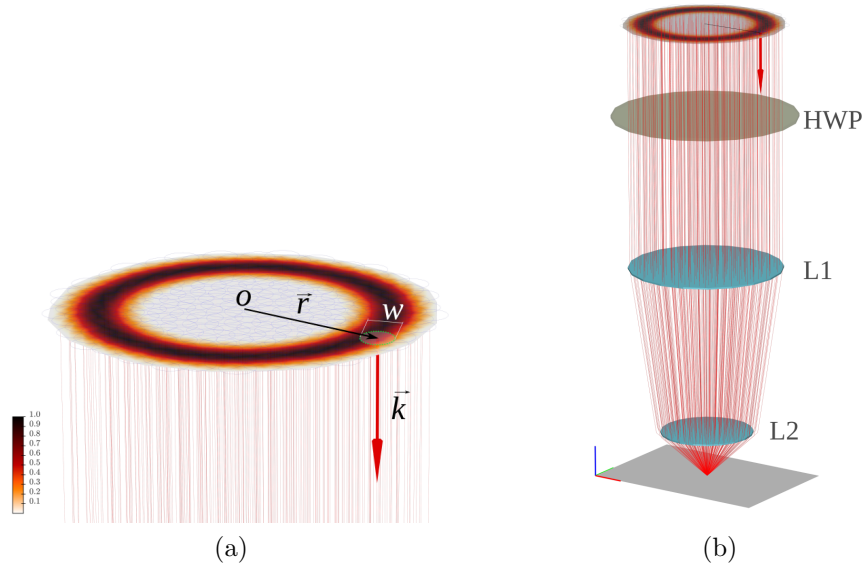

Figure S2: a) Intensity distribution according to the Gaussian beamlet decomposition approach with highlighted single beamlet at position  $\vec{r}$  oriented in direction  $\vec{k}$  and characterized by width  $w$ . b) Visualization of raytracing for incident light propagating through half-wave plate HWP and objective, which is modelled by the combination of thin lenses L1 and L2.

The input laser beam will be constructed as a set of evenly distributed Gaussian beamlets on the grid  $\vec{r}^0$  (see Fig. S2). For grid sampling we will use hexapolar approach.<sup>S8</sup> Each beamlet will carry the information about the local curvature of the wavefront, polarization, amplitude of the field, and phase. Direction of propagation will be defined by the unit wave vector  $\hat{k}^0 = (0, 0, -1)^T$ . The local information about the wavefront will be handled by the complex beam parameter  $q^0$  that can be calculated from the curvature of the front  $\tilde{R}$ , wavelength  $\lambda$ , and width of the beamlet  $w$ :

$$\frac{1}{q} = \frac{1}{\tilde{R}} + \frac{i\lambda}{\pi n w^2}. \quad (20)$$

For the value of width  $w$ , we will use the average distance between the beamlets that corresponds to the overlap factor 2 in the Gaussian beamlet decomposition.

Each beamlet will carry the electrical field vector  $\vec{\mathcal{E}} = (1, 0, 0)^T$  defined in the laboratory coordinate system. For CW excitation regime vector  $\vec{\mathcal{E}}$  will oscillate with angular frequency  $\omega$ :

$$\vec{E}^0 = \vec{\mathcal{E}} e^{-i\omega t}. \quad (21)$$

CW regime allows us to consider only one period of the wave, where the number of samples can be reduced according to Nyquist–Shannon theorem.<sup>S9</sup>

In case of pulsed laser excitation with pulse duration  $\tau$ , the electrical field amplitude will be additionally modulated in time with Gaussian temporal profile for simplicity:

$$\vec{E}^0 = \vec{\mathcal{E}} e^{i\omega t} \exp \left[ -2 \ln(2) \left( \frac{t}{\tau} \right)^2 \right]. \quad (22)$$

This regime requires calculation of the field in a temporal range larger than  $[-\tau, \tau]$  with the same minimal sampling rule as for CW case.

To propagate the beamlet in space from position  $\vec{r}^m$  to the next optical element with

normal  $\hat{N}^{m+1}$  and position  $\tilde{r}^{m+1}$  we need to calculate the distance  $l^{m,m+1}$ :

$$l^{m,m+1} = \mathcal{L}(\tilde{r}^m, \hat{k}^m, \tilde{r}^{m+1}, \hat{N}^{m+1}), \quad (23)$$

$$\mathcal{L}(\vec{a}, \hat{v}, \vec{b}, \hat{n}) = \frac{(\vec{b} - \vec{a}) \cdot \hat{n}}{\hat{v} \cdot \hat{n}}. \quad (24)$$

New position of the beamlet  $\tilde{r}^{m+1}$  and complex parameter  $q^{m+1}$  can be expressed as:

$$\tilde{r}^{m+1} = \tilde{r}^m + \hat{k} l^{m,m+1}, \quad (25)$$

$$q^{m+1} = q^m + l^{m,m+1}. \quad (26)$$

Field  $\vec{E}^{m+1}$  can be obtained by Eq. 13 with  $\tilde{P}$  equal to identity matrix .

Rotation of polarization by angle  $\phi$  is performed by a half-wave plate that can be represented by  $J^{HWP}$  matrix:

$$J^{HWP} = \begin{pmatrix} 1 & 0 \\ 0 & -1 \end{pmatrix} \quad (27)$$

Matrix  $P^{HWP}$  constructed according to Eq. 2 has to be rotated by angle  $\phi/2$ . In our geometry, it corresponds to rotation around  $\hat{Z}$  axis as described in Eq. 6 with rotation matrix  $R^z$ :

$$R^z(\theta) = \begin{pmatrix} \cos \theta & -\sin \theta & 0 \\ \sin \theta & \cos \theta & 0 \\ 0 & 0 & 1 \end{pmatrix} \quad (28)$$

Rotated  $\vec{E}^1$  field can be calculated with Eq. 2

Next step is to propagate polarized beamlets through the objective. For correct calculations, one would need to know the exact design of the optical system with curvatures and refractive indices for each lens. With this information it is possible to propagate the beamlets with use of  $P$  matrix for refraction transformed according to Eq. 6. For simplicity and

fast calculation we will represent the objective as two thin lenses positioned at the entrance and exit pupils. This can be modeled with matrix  $\mathcal{F}$  for the thin lens and matrix  $\mathcal{S}$  for free space propagation:

$$\mathcal{S}(d) = \begin{pmatrix} 1 & d \\ 0 & 1 \end{pmatrix}, \quad (29)$$

$$\mathcal{F}(f) = \begin{pmatrix} 1 & 0 \\ \frac{-1}{f} & 1 \end{pmatrix}, \quad (30)$$

where  $d$  - distance that light propagates in space,  $f$  - focal distance of the thin lens.

Beamlet has to be propagated with Eq. 2 to the entrance pupil of the objective positioned at  $p$  with orthogonal basis  $B = (b^0, b^1, b^2)$ . Vector  $\vec{r}^2$  has to be projected on the plane of the entrance pupil to vector  $\check{r} = (B^{-1}\vec{r}^2)_{0,1}$  and angles  $\check{\theta}$  can be calculated from  $\hat{k}^2$ :

$$k_i^r = |k_i - b_j^2 k_j^2 b_i^2| \quad (31)$$

$$\check{\theta}_{0,1} = \cos^{-1}(k_i^r B_{ij})_{0,1} \quad (32)$$

This allows us to form real  $[\check{r}^0, \tan \check{\theta}^0]$  and complex  $[\check{q}^0, 1]$  ABCD rays and propagate

115 them through the system:

$$\begin{bmatrix} \check{r}^1 \\ \tan \check{\theta}^1 \end{bmatrix} = \mathcal{S}(D)\mathcal{F}(D) \begin{bmatrix} \check{r}^0 \\ \tan \check{\theta}^0 \end{bmatrix}, \quad (33)$$

$$\begin{bmatrix} \check{q}^1 u^1 \\ u^1 \end{bmatrix} = \mathcal{S}(D)\mathcal{F}(D) \begin{bmatrix} \check{q}^0 \\ 1 \end{bmatrix}, \quad (34)$$

$$\begin{bmatrix} \check{r}^2 \\ \tan \check{\theta}^2 \end{bmatrix} = \mathcal{S}(D_{\text{WD}})\mathcal{F}(F) \begin{bmatrix} \check{r}^1 \\ \tan \check{\theta}^1 \end{bmatrix}, \quad (35)$$

$$\begin{bmatrix} \check{q}^2 u^2 \\ u^2 \end{bmatrix} = \mathcal{S}(D_{\text{WD}})\mathcal{F}(F) \begin{bmatrix} \check{q}^1 u^1 \\ u^1 \end{bmatrix}, \quad (36)$$

116 where  $D = D_{\text{PF}} - D_{\text{WD}}$ ,  $D_{\text{PF}}$  - parfocal distance,  $D_{\text{WD}}$  - working distance,  $F = R_1 D D_{\text{WD}} (R_0 D_{\text{WD}} -$   
 117  $R_1 D_{\text{PF}})^{-1}$ ,  $R_0$  and  $R_1$  - entrance and exit pupil radii. Parameter  $u$  is the normalization fac-  
 118 tor.

119 Result of ABCD ray tracing can be mapped to the 3D coordinates as follows:

$$\vec{r}^3 = B (\check{r}^1, 0)^T + b^2 D + p, \quad (37)$$

$$\vec{r}^4 = B (\check{r}^2, 0)^T + b^2 (D + D_{\text{WD}}) + p, \quad (38)$$

$$\vec{k}^3 = |[W(b^0, \check{\theta}_1^1) b^1] \hat{\times} [W(b^1, \check{\theta}_0^1) b^0]|, \quad (39)$$

$$\vec{k}^4 = |[W(b^0, \check{\theta}_1^2) b^1] \hat{\times} [W(b^1, \check{\theta}_0^2) b^0]|, \quad (40)$$

$$(41)$$

120 where  $W$  is the Rodrigues rotation matrix:

$$W(\vec{v}, \theta) = e^{\theta \vec{v}}. \quad (42)$$

121 For each plane, we can calculate the optical path as the difference of the consequent

ray positions. In a real objective, the design of the optical system is optimized to provide minimal wavefront distortion with almost the same arrival time at the focal plane for each input ray. As we use thin lenses, which do not preserve the optical path on the lens itself, an additional correction is needed:

$$OPL^{corr}(f_{eff}, \vec{r}^i, \vec{r}^i, \vec{r}^{i+1}) = |\vec{r}^{i+1} - \vec{r}^i| - \left( \sqrt{|\vec{r}^i|^2 - (f_{eff})^2} - f_{eff} \right), \quad (43)$$

where  $f_{eff}$  is the effective focal length of a thin lens which corresponds to distances  $D$  and  $F$  (see Eq. 37-40) for the first and second lens correspondingly.

After tracing the rays through the ABCD system we can propagate the polarized field according to Eq. 2, where  $P$  matrices for each change of wave vector  $\hat{k}^3$  and  $\hat{k}^4$  are constructed according to Eq. 13. This model does not take into account the polarization variations due to the refraction on the coated interfaces of the real lenses of the objective. We can introduce them with the general Jones matrix from Eq. 3. It has to be converted to  $P$  matrix and transformed according Eq. 6 calculated for each beamlet separately. However, as the objective has the radial symmetry that allows to reduce the number of calculations to a set of Jones matrices that are identical for the same distance from the optical axis.

The last ray tracing step is the refraction at the surface of the sample with normal  $N$ . As in a real experiment, the surface of the sample can slightly be tilted, so we need to rotate the default  $\hat{\mathcal{N}} = (0, 0, -1)^T$  with the rotation matrix  $R^N$ :

$$\hat{N} = R^N \hat{\mathcal{N}}, \quad (44)$$

$$R^N = R^y(\beta_0) R^x(\beta_1), \quad (45)$$

$$R^x(\theta) = \begin{pmatrix} 1 & 0 & 0 \\ 0 & \cos \theta & -\sin \theta \\ 0 & \sin \theta & \cos \theta \end{pmatrix}, \quad (46)$$

$$R^y(\theta) = \begin{pmatrix} \cos \theta & 0 & \sin \theta \\ 0 & 1 & 0 \\ -\sin \theta & 0 & \cos \theta \end{pmatrix}, \quad (47)$$

139 where  $\beta_{0,1}$  - small tilt angles.

## 140 Resampling field on the grid

141 To get the field in the region of the waist, we need to interfere the fields from each beamlets  
 142 that we traced before. For the single beamlet at  $\vec{r}$ , the field on the grid  $\vec{\mathcal{D}}$  that lies on the  
 143 plane perpendicular to the  $\hat{k}$  can be calculated as:<sup>S10</sup>

$$U = \frac{U^0}{q} \exp \left( \frac{ik||\vec{r} - \vec{\mathcal{D}}||^2}{2q} \right) \quad (48)$$

$$\vec{E}^{\mathcal{D}} = U \vec{E}, \quad (49)$$

144 where  $k = 2\pi n/\lambda$  is wave number and  $U_0$  is a scalar field amplitude.

145 As our beamlets are tightly focused with a large variation of angles between the surface  
 146 and  $\hat{k}$  vectors, we can't directly resample by the summation of contributions of each beamlet  
 147 on the same grid as  $q$  is not valid outside of the plane perpendicular plane to  $\hat{k}$ . This  
 148 means that to calculate the field an arbitrary point  $a$  outside of the plane  $(\vec{r}, \hat{k})$ , we need to  
 149 propagate the beamlet by  $P$  matrix according to Eq. 13 for optical paths calculated from

distance  $\mathcal{L}(\vec{r}, \hat{k}, \vec{a}, \hat{k})$  and apply Eq. 48 to get the field at this point.

When the contribution from each of  $N$  beamlets on the grid  $\mathcal{G}$  is known, we can get the total field as sum of contribution from each beamlet:

$$E^6(\vec{\mathcal{G}}) = \sum_N U_N(||\vec{r}_N - \vec{\mathcal{G}}||, q_N) E_N^5(\vec{r}_N) \quad (50)$$

It has to be noted that for pulsed excitation we have to resample  $E_N^5$  on the same time scale to perform this summation.

For simplicity we will reuse the position of the rays  $\vec{r}^5$  as sampling grid  $\mathcal{G}$ .

## Calculation of nonlinear polarization

To calculate the response  $P^{NL}$  of the material defined by some tensor  $K_{a\dots z}$  of rank  $V$  in crystal physics coordinate system with basis  $\mathcal{B} = (Z^0, Z^1, Z^2)$ , we need first orient this tensor and get its representation in the laboratory coordinate system  $\mathcal{K}_{a\dots z}$ . This transformation can be performed according to the general transformation approach by Eq. 6 with the rotation matrix  $R^c$ :

$$R^c = R^N R^z(\alpha_2) R^y(\alpha_2) R^x(\alpha_2), \quad (51)$$

where  $\alpha_i$  - rotation angles.

Response of the sample can be written in general as:

$$P_a^{NL} \sim \mathcal{K}_{abc\dots z} \prod_{\alpha=b}^z E_\alpha \quad (52)$$

For SHG and Raman this equation will have the following forms:

$$E_i^{7,SHG} \sim \chi_{ijk}^{(2)} E_j^6 E_k^6, \quad (53)$$

$$E_i^{7,R} \sim \mathcal{R}_{ij} E_j^6, \quad (54)$$

$$(55)$$

165 where  $\chi^{(2)}$  is second order nonlinear susceptibility,  $\mathcal{R}$  - Raman tensor,  $E^R$  - Raman scattering  
 166 field,  $E^{SHG}$  - SHG field.

## 167 **Collection of the emitted signals**

168 Emitted signals have to be projected on the collection direction defined by  $\hat{k}^8$ . In agreement  
 169 with the treatment in Section 2, we interfered electrical field on the same grid of points  
 170  $\vec{r}^5$ , the wave vector for emission  $\hat{k}^8$  in zero approximation will match with excitation wave  
 171 vector  $\hat{k}^5$  for transmission/reflection geometry. Our microscope is designed for epi-detection  
 172 geometry, so we can apply Eq. 18 with inversion of the sign to determine  $\hat{k}^8$ . More precise  
 173 calculation requires calculation of resulting Poynting vector as described in.<sup>S11</sup>

174 The emitted field has to be rejected on the wave vector as follows:

$$E_i^8 = E_i^7 - k_j^8 E_j^7 k_i^8 \quad (56)$$

175 From this point we need to propagate the new beamlets in reverse through the interface  
 176 of the sample and objective in the same way as we delivered light to the sample. For the  
 177 analysis of the polarization state we will use the polarizer with Jones matrix from Eq. 3  
 178 rotated at angle  $\phi$  for parallel and  $\phi + \pi/2$  for crossed configuration. In the case of Raman  
 179 signal that is detected with the spectrometer, the additional propagation through the general  
 180 Jones matrix  $J^D$  is needed as spectrometer strongly distorts the polarization.

181 Finally, the signal can be detected by summation of the resampled fields according to  
 182 Eq. 48 on the pixels of the sensor and calculation of the intensity:

$$I = G |E^\dagger E|^2, \quad (57)$$

183 where  $G$  is spectral sensitivity of the sensor.

### 3 Fitting procedure

The set of free fitting parameters includes components of the nonlinear response tensor (second-order nonlinear susceptibility tensor  $\chi^{(2)}$  for SHG and  $R$  for Raman), Euler (or Tait-Bryan) angles for the orientation of both the crystal axes and the sample surface, the refractive indices of the sample, parameters of the objective, and additional correction factors. Due to the large number of parameters and the likelihood of encountering multiple local optima in the fitting objective space, we utilize a global optimization approach. Specifically, we apply the large-scale multi-objective competitive swarm optimizer LMOCSO,<sup>S12</sup> a multiobjective evolutionary algorithm executed within the distributed, GPU-accelerated EvoX framework,<sup>S13</sup> which efficiently handles simultaneous fitting of polarization-resolved intensities in both parallel and crossed polarization configurations for SHG and Raman.

Multiobjective algorithms like LMOCSO, NSGA-III,<sup>S14</sup> and RVEA<sup>S15</sup> are particularly suitable for this task, as they aim to identify sets of non-dominated solutions that balance the fit across all data inputs without favoring one. This strategy also permits the inclusion of multiple datasets obtained from different sample orientations or measurement geometries in the same model. While the material tensor remains the same for different datasets, the simultaneous multiobjective fitting of all available inputs improves the reliability of the results.

The quality and completeness of the optimization depend on parameter bounds, model complexity, and tuning of algorithm-specific settings (e.g., population size, mutation/crossover rates). The final output may consist of a single optimal solution or a set of equivalent solutions, which must be manually filtered. This filtering involves comparing the reconstructed orientation of the unit cell with known orientation data from optical microscopy.

## 4 Fitting with single crystal orientation

The results for  $\text{LiNbO}_3$  presented in the main text were obtained by running simulations on NVIDIA L40 GPU with  $5 \cdot 10^5$  generations and a population size 600 species that results in  $3 \cdot 10^8$  combination of tested parameters. Figure S3 shows the influence of the constraints on the final population distribution of the main parameters of the model. A strongly constrained model with probing of multiple orientations of the crystal described by the same tensor, provides better precision with narrower population distribution peaks. Although this approach is recommended, it is not always possible to rotate the sample and probe the response from all of the faces. In this case, the precision for each tensor element will depend of the orientation of the crystal and the projection of the induced nonlinear polarization on the detection plane. For demonstration of the performance of MRANHG technique we performed fitting of a single face from LN dataset obtained from  $ab$  face that has to demonstrate the lowest SHG efficiency. From the population distribution we can clearly see the broadening of the peaks, which indicates lower confidence in the result. In case of  $zzz$  there is no clearly defined peak but the result remains close to the constrained model. This fact means that we do not directly read the optimal result for  $zzz$  but reconstruct it from the optimization of the rest of the parameters, as all of the values on the histograms are linked between each other.

## 5 Contracted notation

Many reference papers talk about nonlinear susceptibility tensor  $d_{il}$  ( $3 \times 6$ ) that has reduced dimensionality in comparison with  $\chi_{ijk}^{(2)}$  ( $3 \times 3 \times 3$ ) to simplify the calculation. It becomes useful, when the Kleinman symmetry condition is valid. Tensor  $d_{il}$  can be obtained from  $\chi_{ijk}^{(2)}$  as:

$$d_{il} = \frac{1}{2} \chi_{ijk}^{(2)}, \quad (58)$$

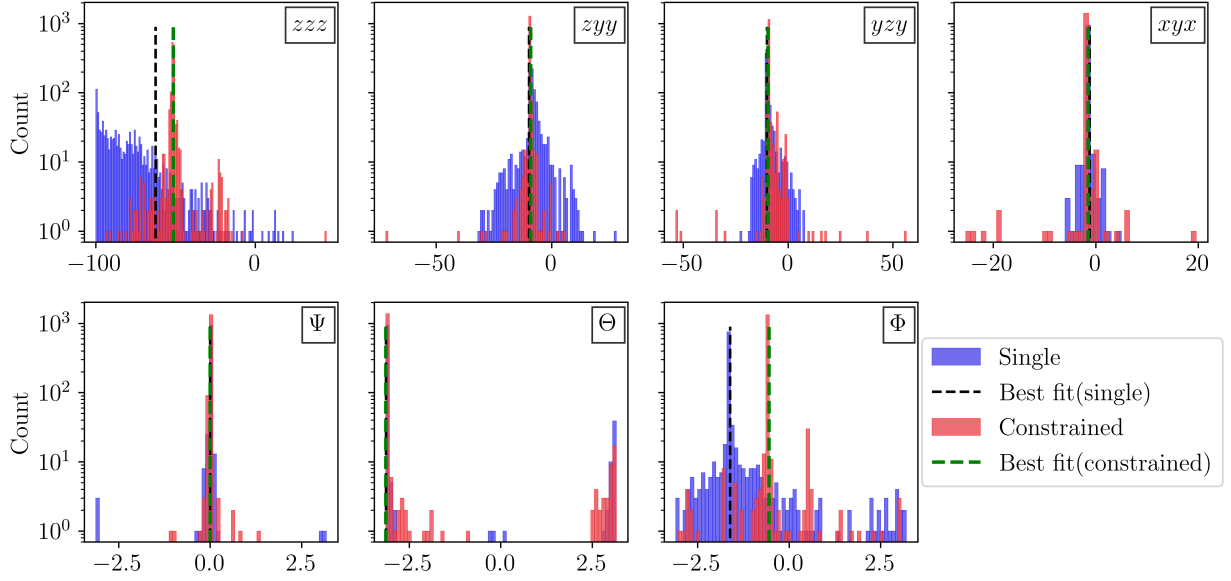

Figure S3: Comparison of optimized populations for main LN parameters:  $zzz$ ,  $zyy$ ,  $yzy$ ,  $xyx$  tensor elements and Tait-Bryan (Cardan) angles  $\Psi$ ,  $\Theta$ ,  $\Phi$ . Results were obtained for single orientation ( $ab$ -plane) and the model constrained by the full set of orientations ( $ab$ ,  $ab$  rotated by  $45^\circ$ , and  $c$ ).

where index  $l$  is defined by contracted notation:

$$\begin{array}{c|cccccc} \text{jk:} & 11 & 22 & 33 & 23,32 & 13,31 & 12,21 \\ \hline \text{l:} & 1 & 2 & 3 & 4 & 5 & 6 \end{array}$$

230

231 According to contraction rule and Kleinman symmetry ( $xzx = yzy, xxz = yyz, zxx =$   
 232  $zyy, zzz, yyy = -yxx = -xxy = -xyx$ ) the  $d_{il}$  tensor for  $\text{LiNbO}_3$  can be written as:<sup>S16</sup>

$$d_{il} = \begin{bmatrix} 0 & 0 & 0 & 0 & d_{32} & -d_{22} \\ -d_{22} & d_{22} & 0 & d_{32} & 0 & 0 \\ d_{31} & d_{31} & d_{33} & 0 & 0 & 0 \end{bmatrix} \quad (59)$$

233 In this paper we work with  $\chi_{ijk}^{(2)}$  tensor that is not optimal in term of calculation time  
 234 but allows to combine the responses for future work.

## References

- (S1) Wende, M.; Drozella, J.; Toulouse, A.; Herkommer, A. M. Fast algorithm for the simulation of 3D-printed microoptics based on the vector wave propagation method. *Optics Express* **2022**, *30*, 40161.
- (S2) Hu, Y.; Wang, Z.; Wang, X.; Ji, S.; Zhang, C.; Li, J.; Zhu, W.; Wu, D.; Chu, J. Efficient full-path optical calculation of scalar and vector diffraction using the Bluestein method. *Light: Science & Applications* **2020**, *9*, 119.
- (S3) Sukhoy, V.; Stoytchev, A. Generalizing the inverse FFT off the unit circle. *Scientific Reports* **2019**, *9*, 14443.
- (S4) Ye, H.; Qiu, C.-W.; Huang, K.; Teng, J.; Luk'yanchuk, B.; Yeo, S. P. Creation of a longitudinally polarized subwavelength hotspot with an ultra-thin planar lens: vectorial Rayleigh–Sommerfeld method. *Laser Physics Letters* **2013**, *10*, 065004.
- (S5) Chipman, R.; Lam, W. S. T.; Young, G. *Polarized light and optical systems*; CRC press, 2018.
- (S6) Born, M.; Wolf, E.; Bhatia, A. B.; Clemmow, P. C.; Gabor, D.; Stokes, A. R.; Taylor, A. M.; Wayman, P. A.; Wilcock, W. L. *Principles of Optics: Electromagnetic Theory of Propagation, Interference and Diffraction of Light*, 7th ed.; Cambridge University Press, 1999.
- (S7) Worku, N.; Gross, H. Vectorial field propagation through high NA objectives using polarized Gaussian beam decomposition. *Optical Trapping and Optical Micromanipulation XIV*. 2017; pp 107–117.
- (S8) Díaz, J. A.; Navarro, R. Geometric optical transfer function and pupil sampling patterns. *Optik* **2023**, *279*, 170746.

- 258 (S9) Luke, H. The origins of the sampling theorem. *IEEE Communications Magazine* **1999**,  
259 37, 106–108.
- 260 (S10) Goodman, J. W. *Introduction to Fourier optics*; Roberts and Company publishers,  
261 2005.
- 262 (S11) Javurek, D.; Peřina Jr, J. Analytical model of surface second-harmonic generation.  
263 *Scientific reports* **2019**, 9, 4679.
- 264 (S12) Tian, Y.; Zheng, X.; Zhang, X.; Jin, Y. Efficient Large-Scale Multiobjective Optimiza-  
265 tion Based on a Competitive Swarm Optimizer. *IEEE Transactions on Cybernetics*  
266 **2020**, 50, 3696–3708.
- 267 (S13) Huang, B.; Cheng, R.; Li, Z.; Jin, Y.; Tan, K. C. EvoX: A Distributed GPU-accelerated  
268 Framework for Scalable Evolutionary Computation. *IEEE Transactions on Evolution-  
269 ary Computation* **2024**,
- 270 (S14) Deb, K.; Jain, H. An evolutionary many-objective optimization algorithm using  
271 reference-point-based nondominated sorting approach, part I: solving problems with  
272 box constraints. *IEEE transactions on evolutionary computation* **2013**, 18, 577–601.
- 273 (S15) Cheng, R.; Jin, Y.; Olhofer, M.; Sendhoff, B. A reference vector guided evolution-  
274 ary algorithm for many-objective optimization. *IEEE transactions on evolutionary  
275 computation* **2016**, 20, 773–791.
- 276 (S16) Boyd, R. W. *Nonlinear optics*, 3rd ed.; Academic Press: Burlington, MA, 2008.
